# Supplementary material for: ClearLines - Camera Calibration from Straight Lines
Source: arXiv:2505.00452 source file (2025-05-01)
Supplement: Supplementary file 1 [file 07_appendix.tex]

\section{Appendix} 
\label{sec:appendix}

% Results EDCircle
%EDCircle performs fantastic at detecting smaller, fully contained circles and ellipses, even in challenging cases and with little false positives. It fails when it comes to fractional arcs though. This did also not improve substantially when decreasing the minimum angle threshold for consecutive lines which we initially assumed to be the reason for the low detection rate. 
%
% We noticed some true positives for arcs in the Omnidirectional SLAM dataset~\cite{2015-LSD-dataset} but those were mostly limited to cases when the corresponding ellipses was not substantially larger than the image. 

%%% Kitti results %%%
\begin{figure*}%[h]%[H]
\subfloat{\includegraphics[height=3.0cm,width=5.8cm]{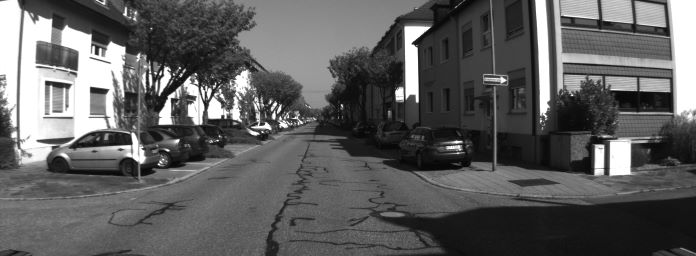}}
\hspace{0.1cm}
\subfloat{\includegraphics[height=3.0cm,width=5.8cm]{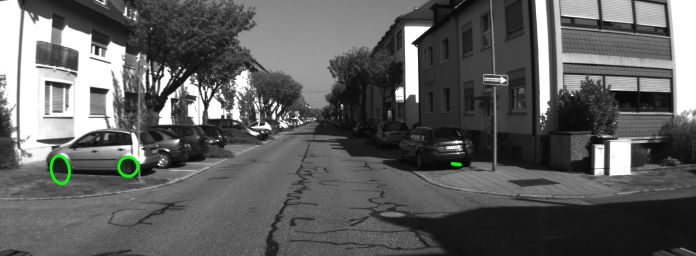}}
\hspace{0.1cm}
\subfloat{\includegraphics[height=3.0cm,width=5.8cm]{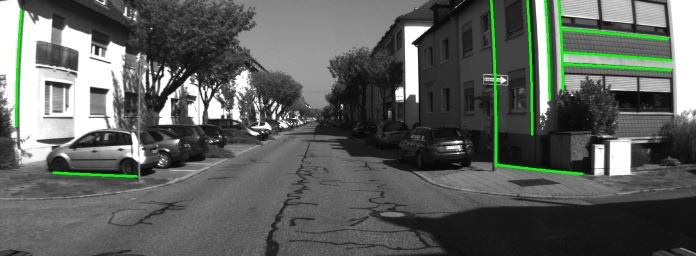}}
\vspace{0.1cm}
\subfloat{\includegraphics[height=3.0cm,width=5.8cm]{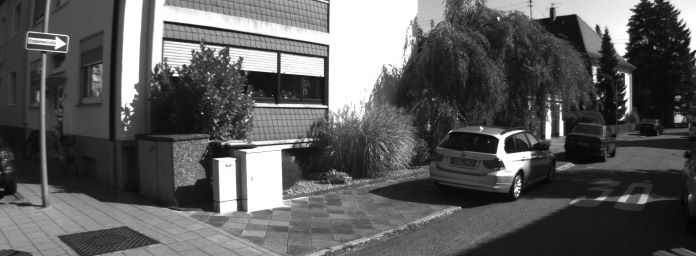}}
\hspace{0.1cm}
\subfloat{\includegraphics[height=3.0cm,width=5.8cm]{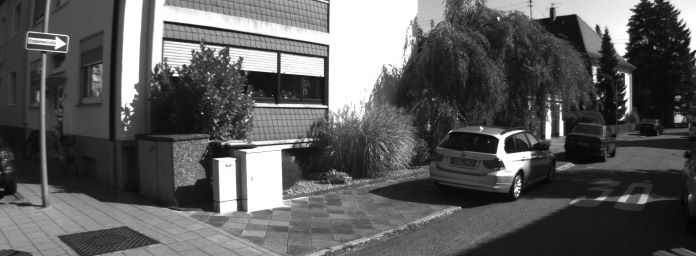}}
\hspace{0.1cm}
\subfloat{\includegraphics[height=3.0cm,width=5.8cm]{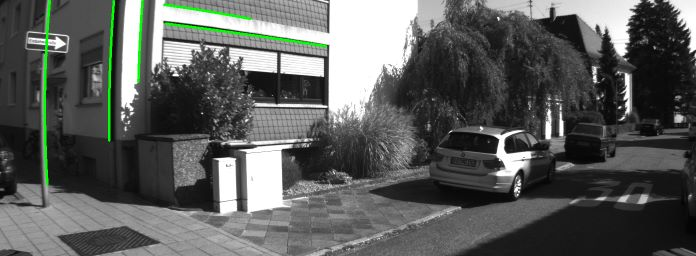}}
\vspace{0.1cm}
\subfloat{\includegraphics[height=3.0cm,width=5.8cm]{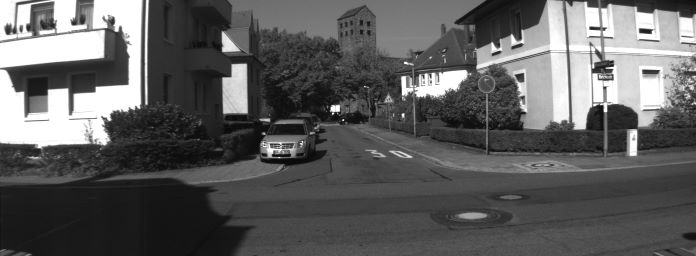}}
\hspace{0.1cm}
\subfloat{\includegraphics[height=3.0cm,width=5.8cm]{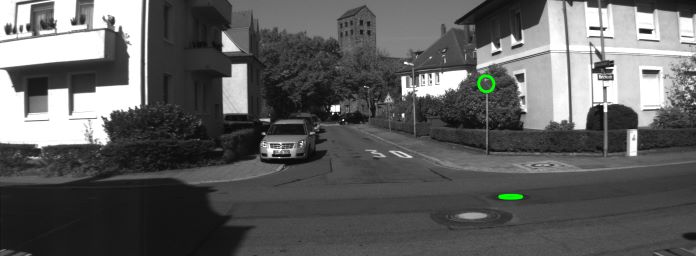}}
\hspace{0.1cm}
\subfloat{\includegraphics[height=3.0cm,width=5.8cm]{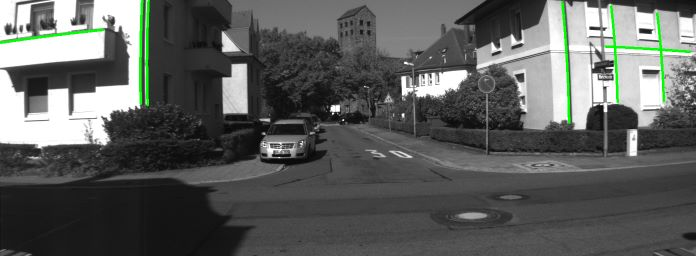}}
\vspace{0.1cm}
\subfloat{\includegraphics[height=3.0cm,width=5.8cm]{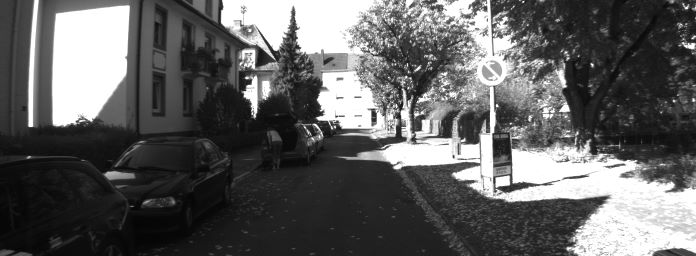}}
\hspace{0.1cm}
\subfloat{\includegraphics[height=3.0cm,width=5.8cm]{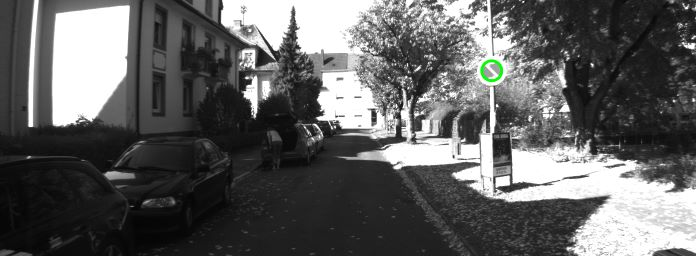}}
\hspace{0.1cm}
\subfloat{\includegraphics[height=3.0cm,width=5.8cm]{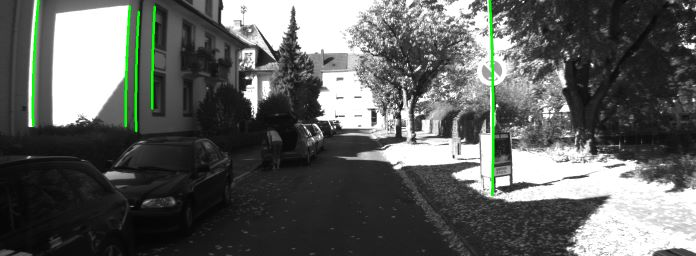}}
\vspace{0.1cm}
\subfloat{\includegraphics[height=3.0cm,width=5.8cm]{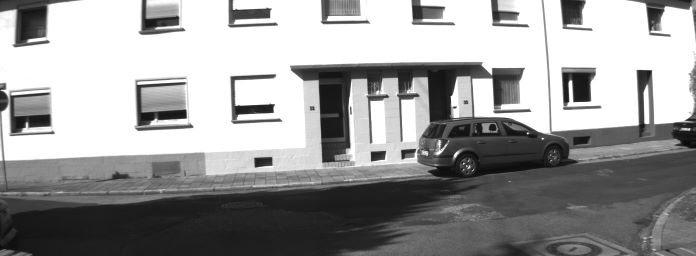}}
\hspace{0.1cm}
\subfloat{\includegraphics[height=3.0cm,width=5.8cm]{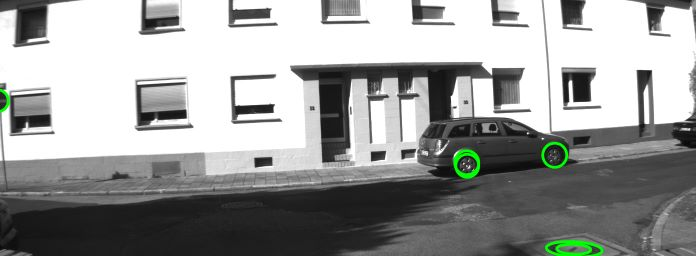}}
\hspace{0.1cm}
\subfloat{\includegraphics[height=3.0cm,width=5.8cm]{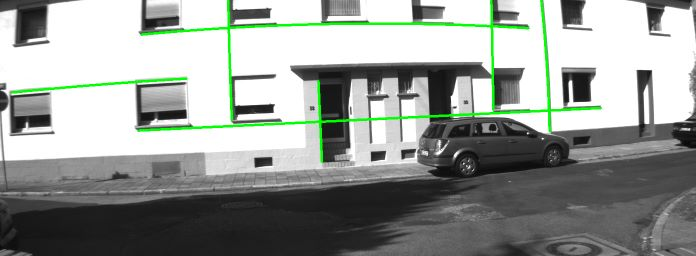}}
%
%\vspace{0.1cm}
%\subfloat{\includegraphics[height=3.0cm,width=5.8cm]{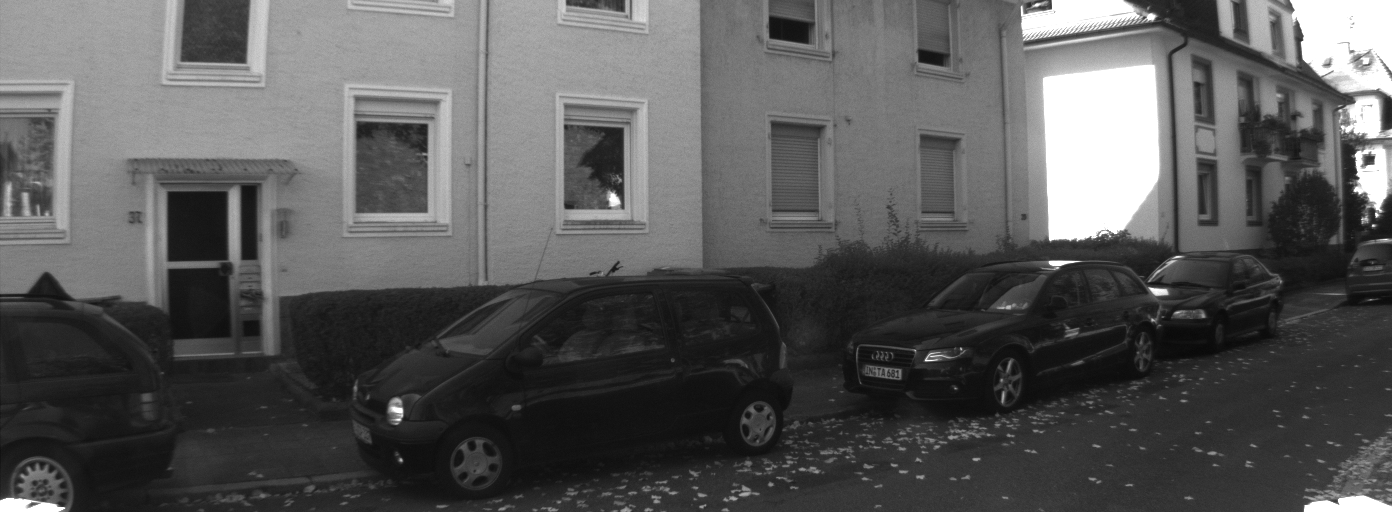}}
%\hspace{0.1cm}
%\subfloat{\includegraphics[height=3.0cm,width=5.8cm]{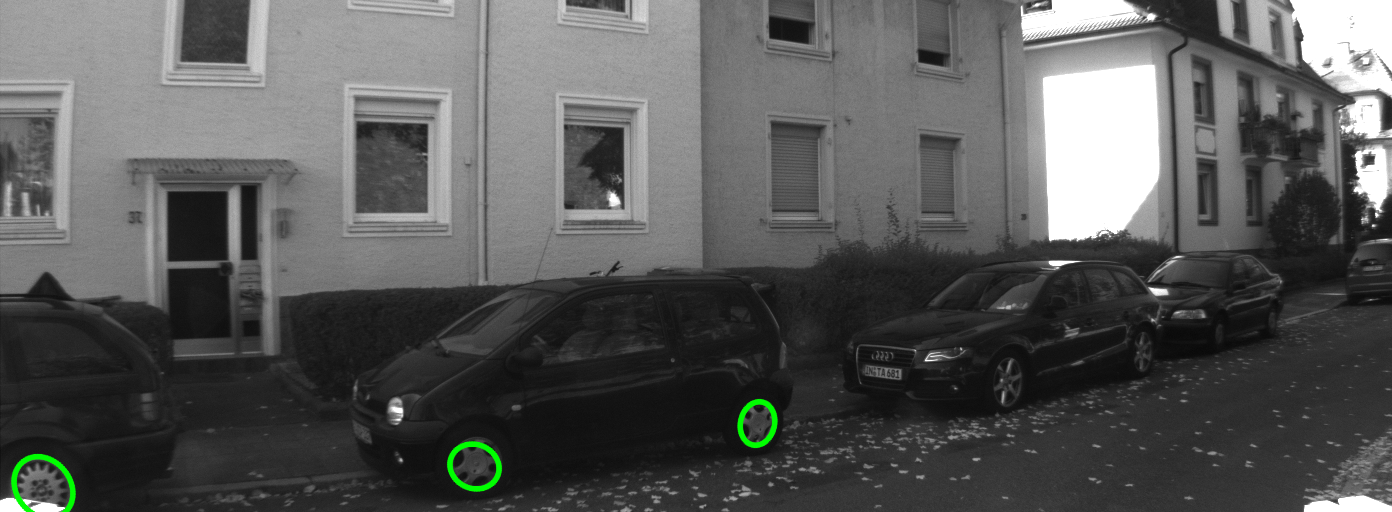}}
%\hspace{0.1cm}
%\subfloat{\includegraphics[height=3.0cm,width=5.8cm]{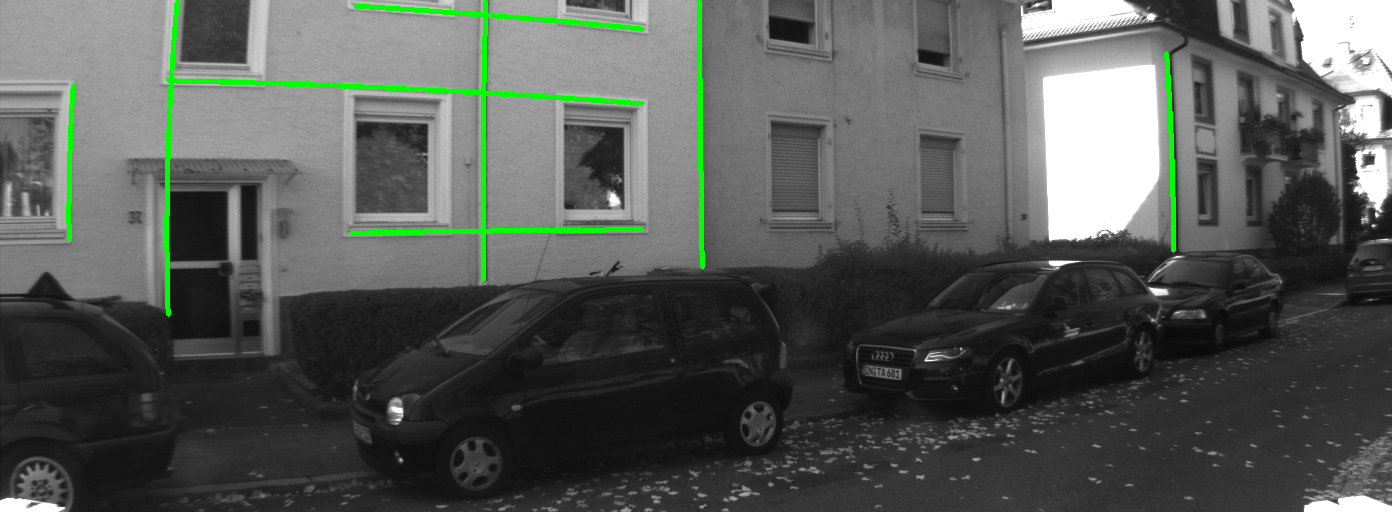}}
%
\vspace{0.1cm}
\subfloat[Input images from \cite{2013-kitti-dataset}]{\includegraphics[height=3.0cm,width=5.8cm]{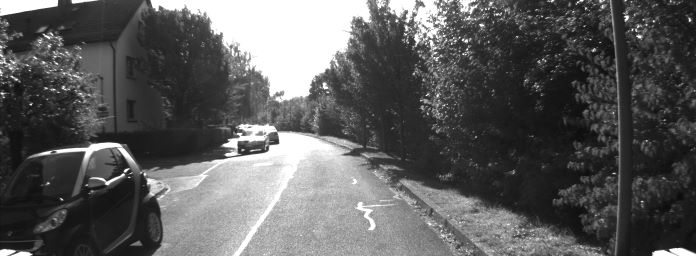}}
\hspace{0.1cm}
\subfloat[EDCircle~\cite{2013_EDcircle_detect}]{\includegraphics[height=3.0cm,width=5.8cm]{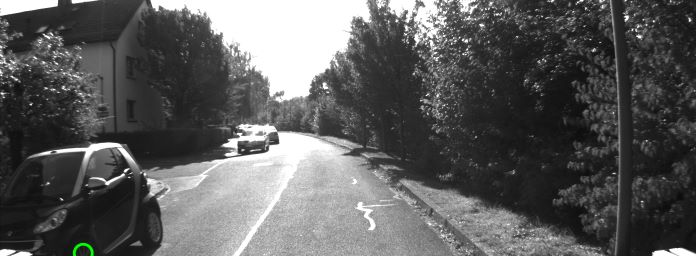}}
\hspace{0.1cm}
\subfloat[Our approach]{\includegraphics[height=3.0cm,width=5.8cm]{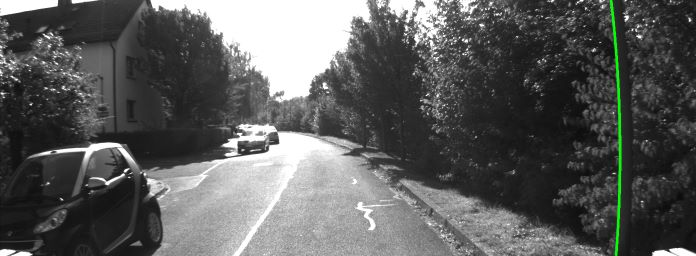}}
\caption{Results our approach vs EDCircle~\cite{2013-EDcircle-detect} for the Kitti dataset~\cite{2013-kitti-dataset}. EDCircle performs fantastic at detecting smaller, fully contained circles and ellipses, even in challenging cases and with little false positives. It fails when it comes to fractional arcs though. This did also not improve substantially when decreasing the minimum angle threshold for consecutive lines which we initially assumed to be the reason for the low detection rate.}
\label{fig:results_kitti_seq00}
\end{figure*}

%%% LSD results %%%
\begin{figure*}%[h]%[H]
\subfloat{\includegraphics[height=3.0cm,width=5.8cm]{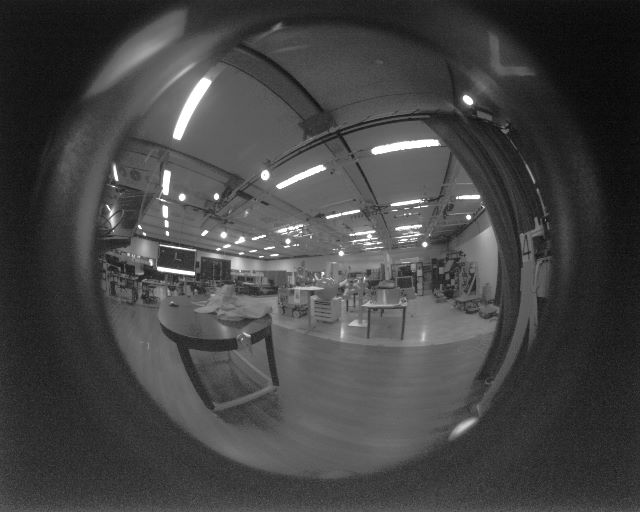}}
\hspace{0.1cm}
\subfloat{\includegraphics[height=3.0cm,width=5.8cm]{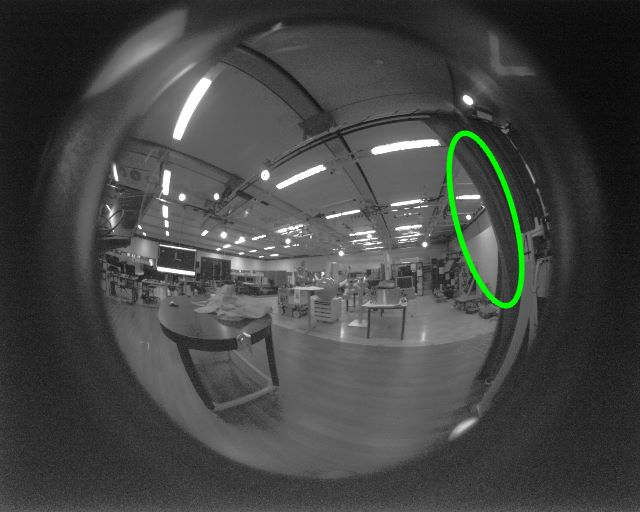}}
\hspace{0.1cm}
\subfloat{\includegraphics[height=3.0cm,width=5.8cm]{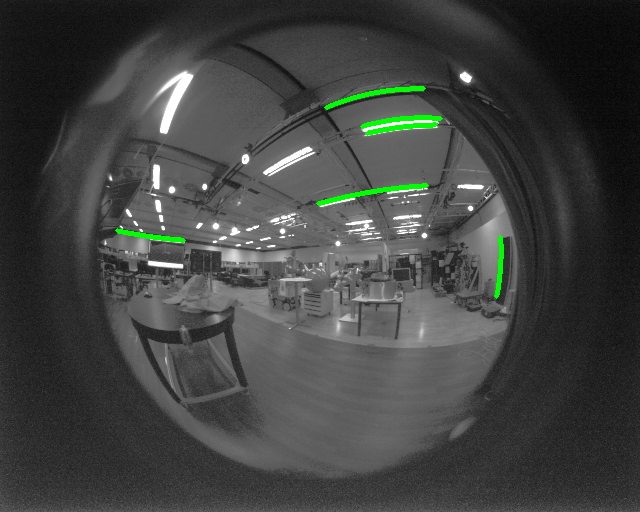}}
\vspace{0.1cm}
\subfloat{\includegraphics[height=3.0cm,width=5.8cm]{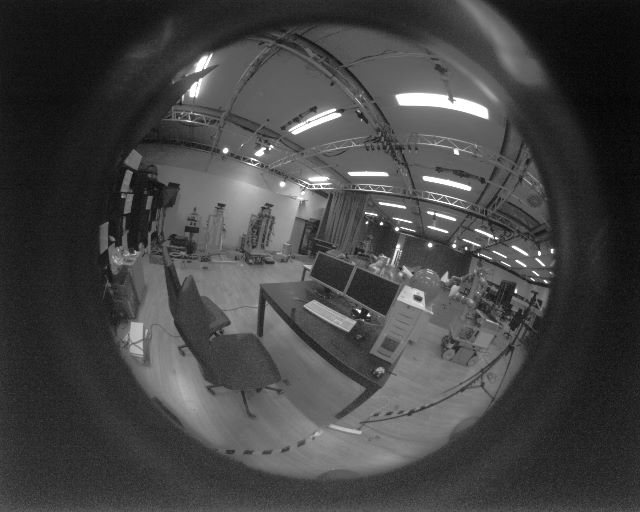}}
\hspace{0.1cm}
\subfloat{\includegraphics[height=3.0cm,width=5.8cm]{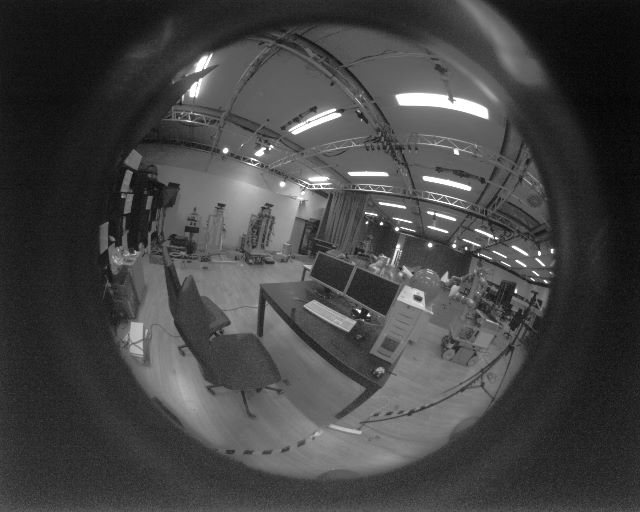}}
\hspace{0.1cm}
\subfloat{\includegraphics[height=3.0cm,width=5.8cm]{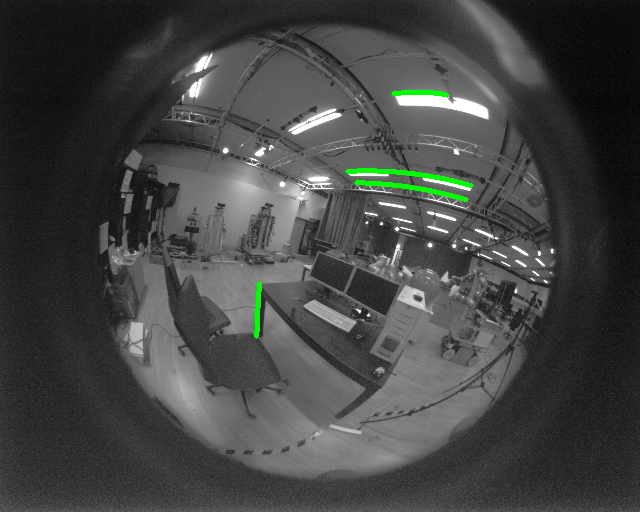}}
\vspace{0.1cm}
\subfloat{\includegraphics[height=3.0cm,width=5.8cm]{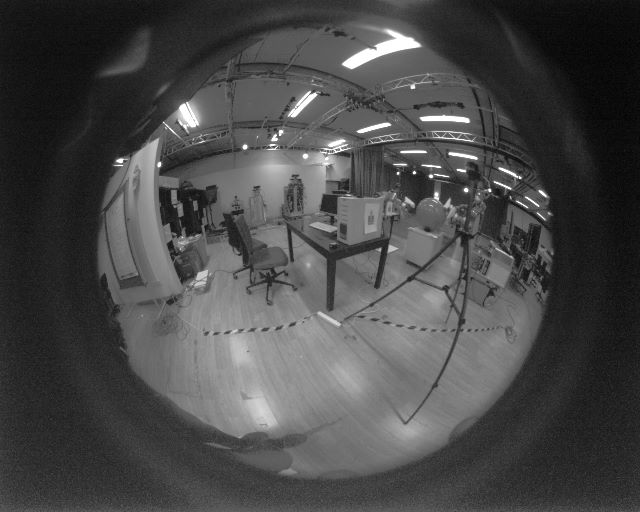}}
\hspace{0.1cm}
\subfloat{\includegraphics[height=3.0cm,width=5.8cm]{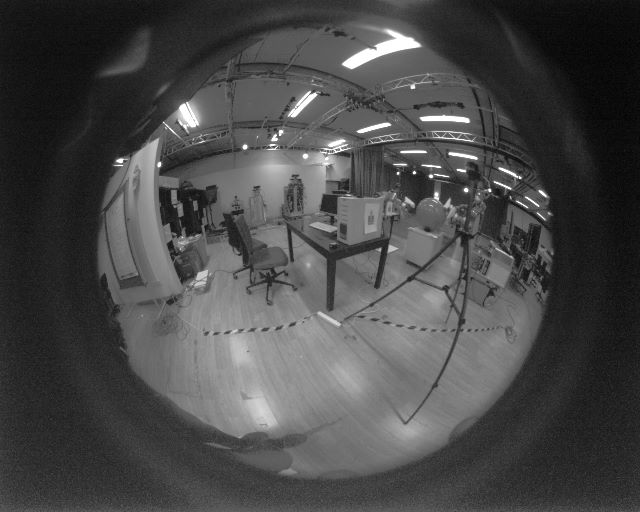}}
\hspace{0.1cm}
\subfloat{\includegraphics[height=3.0cm,width=5.8cm]{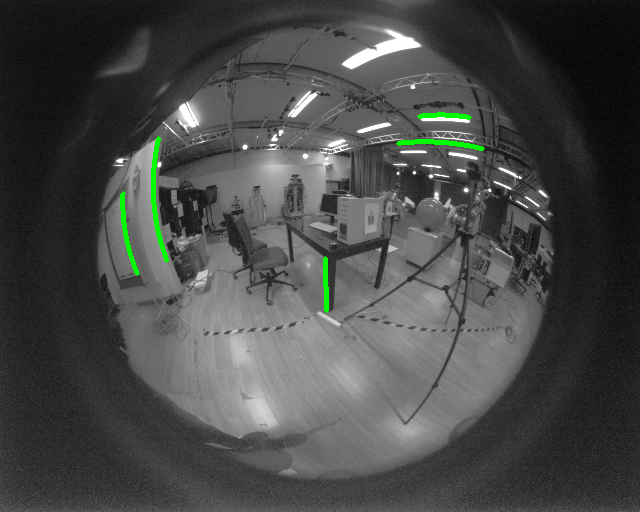}}
\vspace{0.1cm}
\subfloat{\includegraphics[height=3.0cm,width=5.8cm]{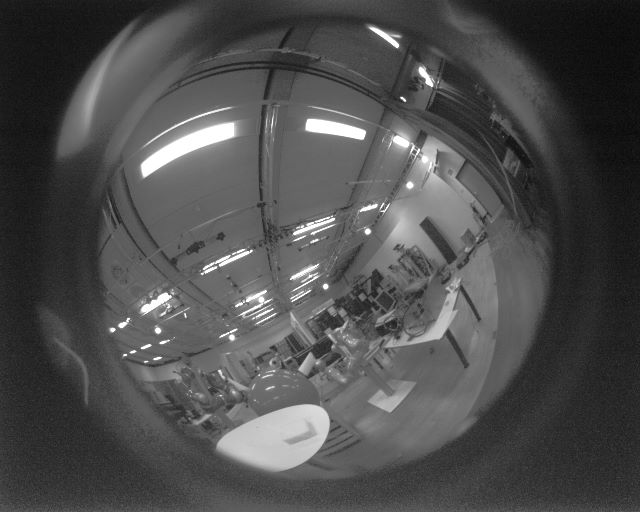}}
\hspace{0.1cm}
\subfloat{\includegraphics[height=3.0cm,width=5.8cm]{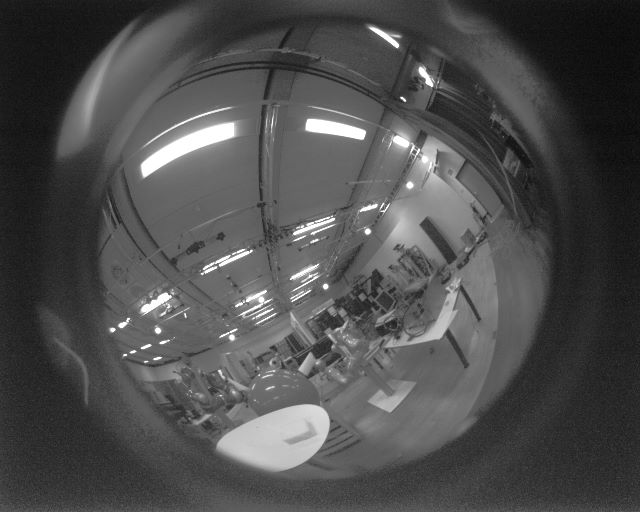}}
\hspace{0.1cm}
\subfloat{\includegraphics[height=3.0cm,width=5.8cm]{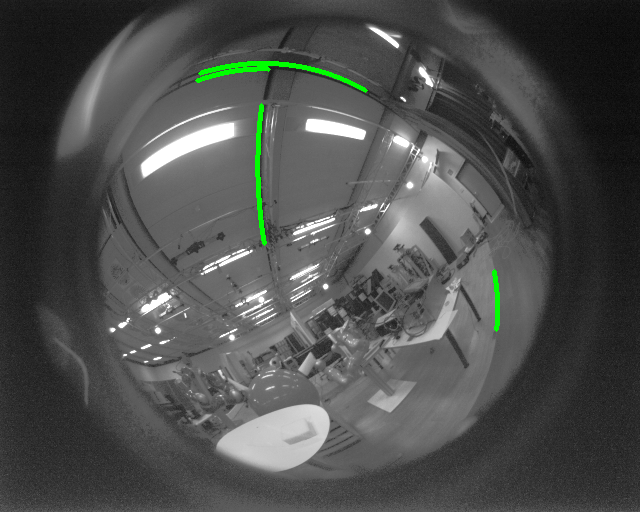}}
\vspace{0.1cm}
\subfloat{\includegraphics[height=3.0cm,width=5.8cm]{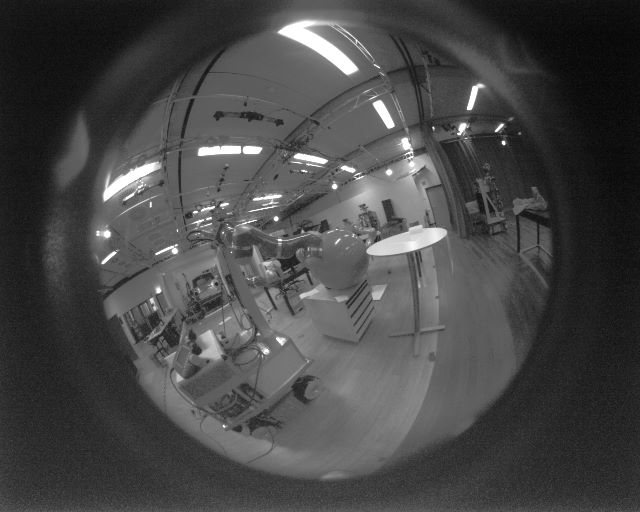}}
\hspace{0.1cm}
\subfloat{\includegraphics[height=3.0cm,width=5.8cm]{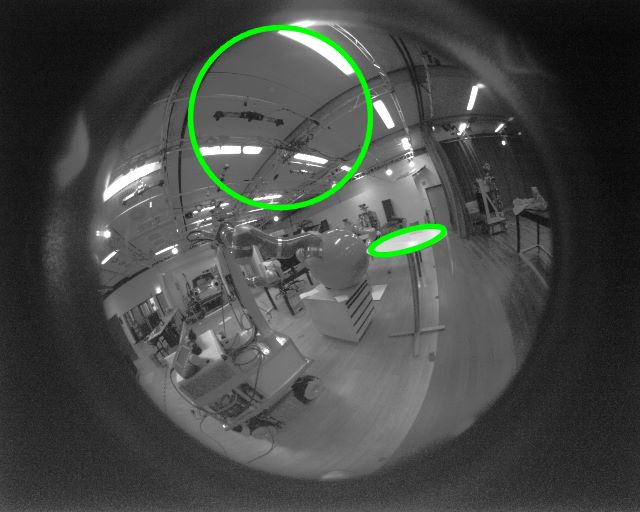}}
\hspace{0.1cm}
\subfloat{\includegraphics[height=3.0cm,width=5.8cm]{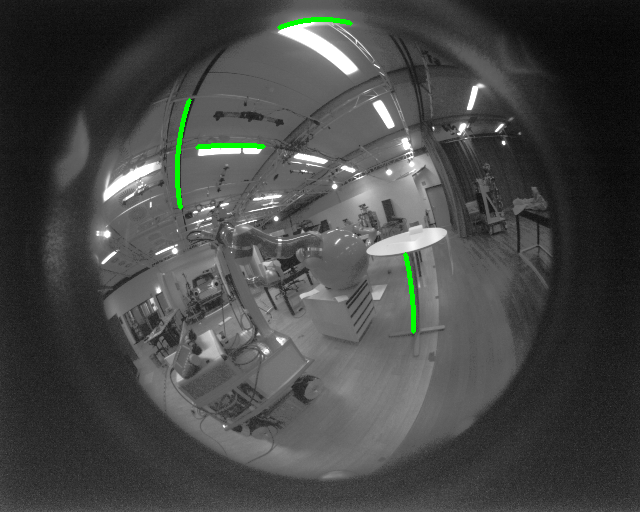}}
\vspace{0.1cm}
\subfloat[Input images from \cite{2015_LSD_dataset}]{\includegraphics[height=3.0cm,width=5.8cm]{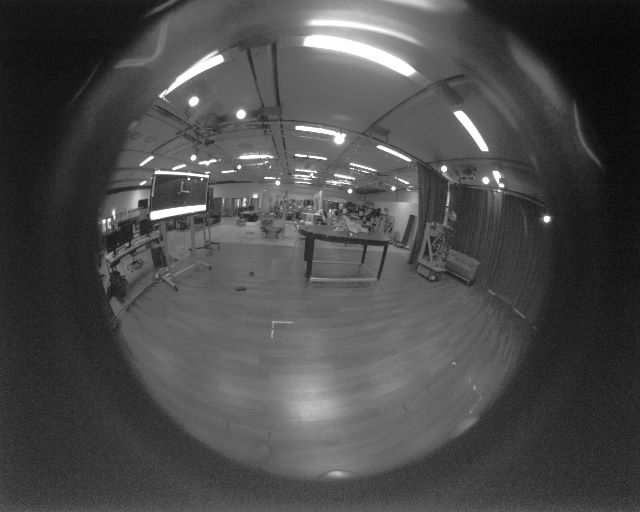}}
\hspace{0.1cm}
\subfloat[EDCircle~\cite{2013_EDcircle_detect}]{\includegraphics[height=3.0cm,width=5.8cm]{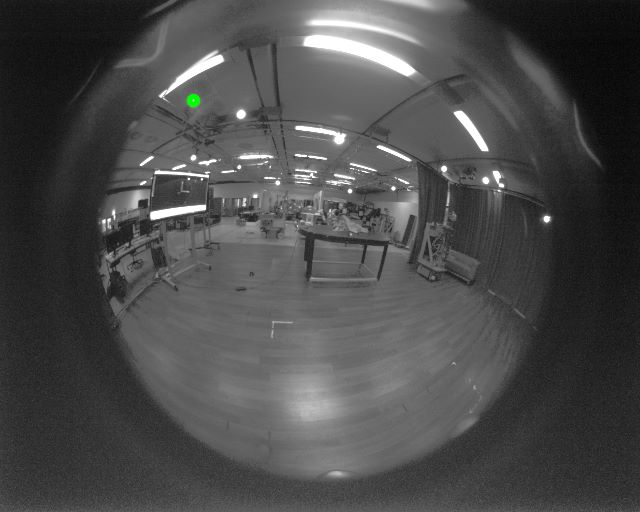}}
\hspace{0.1cm}
\subfloat[Our approach]{\includegraphics[height=3.0cm,width=5.8cm]{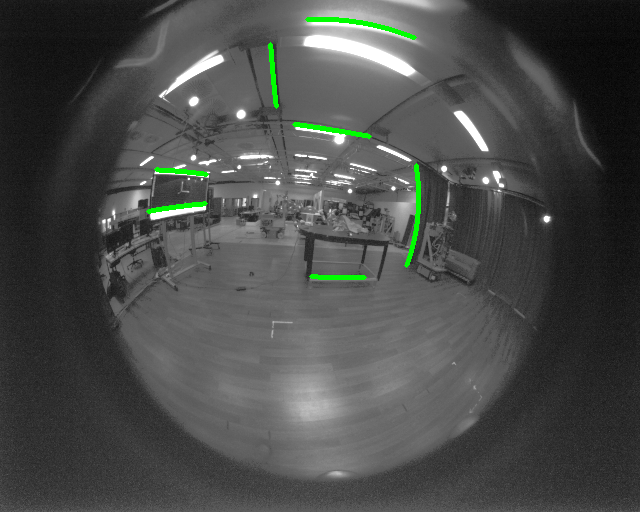}}
\caption{Results our approach vs EDCircle~\cite{2013-EDcircle-detect} for the Omnidirectional SLAM dataset~\cite{2015-LSD-dataset}. We noticed some true positives for arcs from EDCircle but those were mostly limited to cases when the corresponding ellipses was not substantially larger than the image. }
\label{fig:results_LSD}
\end{figure*}
